# Supplementary material for: A Pain Assessment Framework based on multimodal data and Deep Machine Learning methods
Source: arXiv:2505.05396 source file (2025-05-11)
Supplement: Supplementary file 2 [file appendix_metrics.tex]

\phantomsection
\section*{Supplementary Metrics}
\label{appendix_metrics}
